# Supplementary material for: Field-Emission Resonances in Thin Metallic Films: Nonexponential Decay of the Tunneling Current as a Function of the Sample-to-Tip Distance
Source: arXiv:2308.00418 source file (2023-08-01)
Supplement: Supplementary file 1 [file Aladyshkin_SupplementMaterial_v3.pdf]

## Supporting Information

### Field-Emission Resonances in Thin Metallic Films: Non-Exponential Decrease of the Tunneling Current as a Function of the Sample-to-Tip Distance

Alexey Yu. Aladyshkin<sup>(1,2,3,\*)</sup> and Koen Schouteden<sup>(4)</sup>

<sup>(1)</sup> *Institute for Physics of Microstructures RAS, GSP-105, Nizhny Novgorod, 603950 Russia*

<sup>(2)</sup> *Lobachevsky State University of Nizhny Novgorod, Gagarin Avenue 23, Nizhny Novgorod, 603022 Russia*

<sup>(3)</sup> *National Research University Higher School of Economics (HSE University),  
Myasnitskaya str. 20, 101000 Moscow, Russia*

<sup>(4)</sup> *Semiconductor Physics Section, Katholieke Universiteit Leuven, Celestijnenlaan 200D, B-3001 Leuven, Belgium*

<sup>(\*)</sup> E-mail: aladyshkin@ipmr.ru

## Quantum-confined states in a one-dimensional potential well

It is illustrative to consider a model problem of the formation of localized electronic states in asymmetric one-dimensional (1D) potential well

$$-\frac{\hbar^2}{2m^*} \frac{d^2}{dz^2} \psi_n(z) + U(z) \psi_n(z) = E_n \psi_n(z), \quad (\text{S1})$$

where  $\psi_n(z)$  and  $E_n$  are the eigenfunctions and eigenvalues of the Schrödinger equation,  $U(z)$  is the potential energy. For simplicity we take periodic potential inside the quantum well in the form of a combination of two Fourier components

$$U(z) = \begin{cases} U_{left} & \text{for } z < -L/2; \\ U_0 + U_1 \cdot \cos(2\pi z/a) + U_2 \cdot \cos(4\pi z/a) & \text{for } -L/2 \leq z \leq L/2; \\ U_{right} & \text{for } z > L/2, \end{cases} \quad (\text{S2})$$

where  $a$  is the lattice parameter,  $L$  – width of the quantum well. Two Fourier-components of the potential ensure the formation of two forbidden gaps in the spectrum of the electronic eigenstates.

The results of direct numerical solution of Eq. (S1) for the potential well with almost symmetrical edges ( $U_{left} = 0$  and  $U_{right} \simeq 0$ ) are presented in figure S1. One can see that the periodic potential induces well-known Tamm-Shockley states localized near the edges of the crystal with energies lying in the forbidden gaps. Figure S2 demonstrates the modification of both eigenfunctions and eigenvalues caused by a Coulomb-like potential near the right edge of the crystal ( $U_{right} \simeq \text{const}_1 - \text{const}_2/(z - L/2)$ , panel a) and by a linearly increasing potential near the right edge of the crystal ( $U_{right} \simeq \text{const}_1 + \text{const}_2 \cdot (z - L/2)$ , panel b) without taking into account the effect of the image potential.

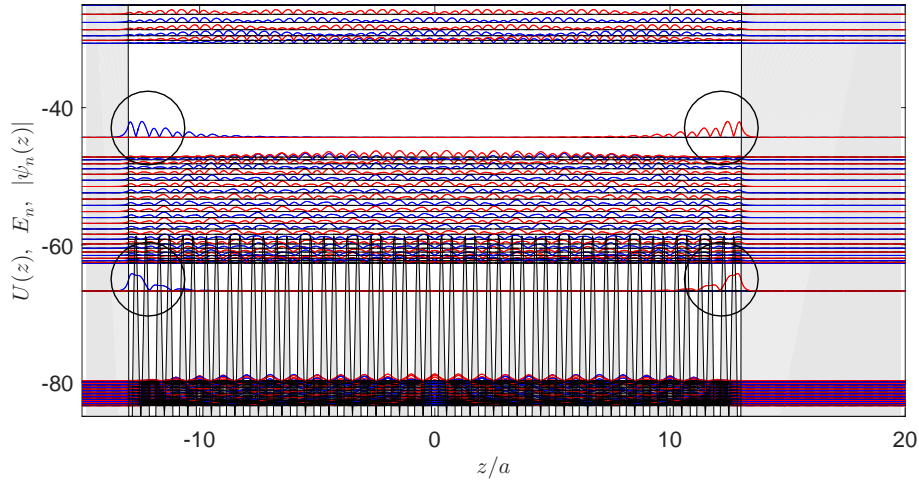

**Figure S1.** (color online) Examples of the stationary eigenfunctions  $|\psi_n(z)|$  of Eq. (S1) for one-dimensional quantum well with almost symmetric edges:  $U_0 = -8E_0$ ,  $U_1 = -0.5E_0$ ,  $U_2 = -0.5E_0$ , where  $E_0 = \pi^2\hbar^2/(2m_0a^2)$ . All these eigenfunctions are shifted vertically with respect to their eigenvalues  $E_n$ . A concentration of the eigenvalues points to an allowed energy bands. Large circles mark the Tamm-Shockley surface states lying within the first and the second forbidden gaps of the bulk crystal.

It allows us to conclude that all types of considered surface states (namely, classical Tamm-Shockley states, image-potential states and states localized in a linearly increasing potential) are the same from the physical point of view. It is clear that the energies and the spatial structure of the wave functions of the localized states are sensitive to the profile of the potential energy outside the potential well.

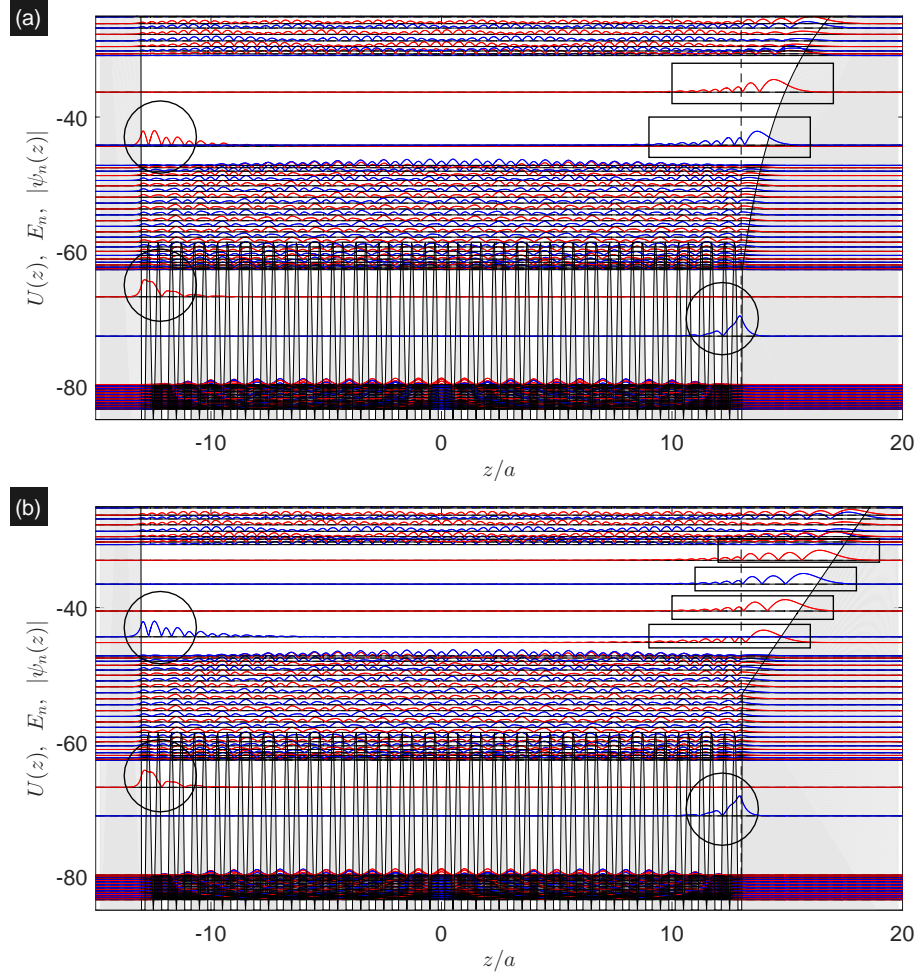

**Figure S2.** (color online) (a) Examples of the stationary eigenfunctions of Eq. (S1)  $|\psi_n(z)|$  for one-dimensional quantum well with non-symmetric edges and Coulomb potential near the right edge (panel a) or linearly-increasing electric potential near the right edge (panel b):  $U_0 = -8 E_0$ ,  $U_1 = -0.5 E_0$ ,  $U_2 = -0.5 E_0$ , where  $E_0 = \pi^2 \hbar^2 / (2m_0 a^2)$ . All these eigenfunctions are shifted vertically with respect to their eigenvalues  $E_n$ . Large circles mark the classical Tamm-Shockley surface states lying within the first and the second forbidden gaps of the bulk crystal, while rectangles depict image-potential states (panel a) and Stark-shifted image-potential states (panel b) in the second forbidden gap.

# The principle of the mutual adjustment of the $Z - U$ and $I - \Delta Z$ dependences

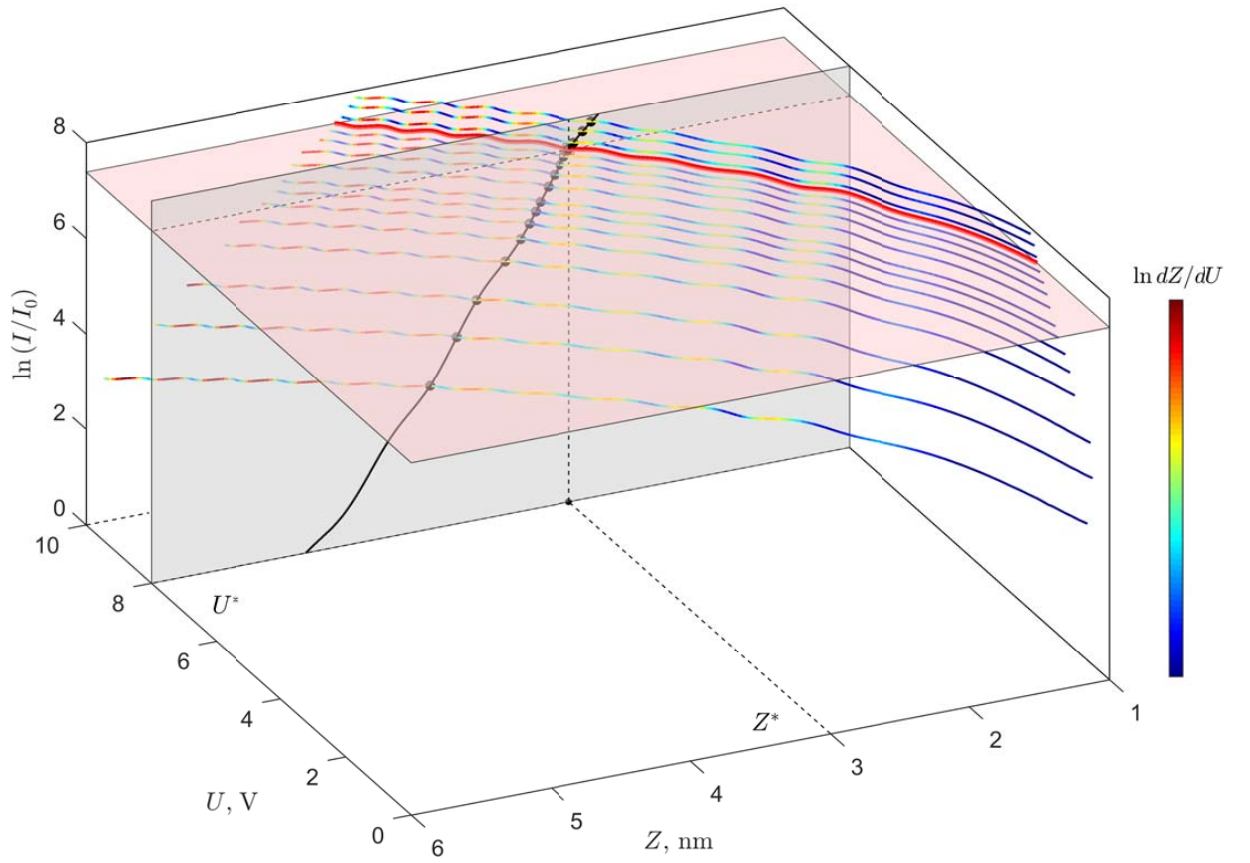

**Figure S3.** (color online) Diagrams illustrating the principle of the mutual adjustment of the  $Z - U$  dependences acquired in the regime of constant current and  $I - Z$  dependences acquired in the regime of constant voltage in a 3D geometry. This particular adjustment is carried out for the following values:  $U^* = 8 V$ ,  $I^* = 1600 pA$ ,  $Z^* = 3 nm$ ,  $I_0 = 1 pA$ . Color of all points is proportional to  $\ln dZ/dU$ . The same plot in 2D geometry is presented in Fig. S4 and Fig. 4a of the main paper.

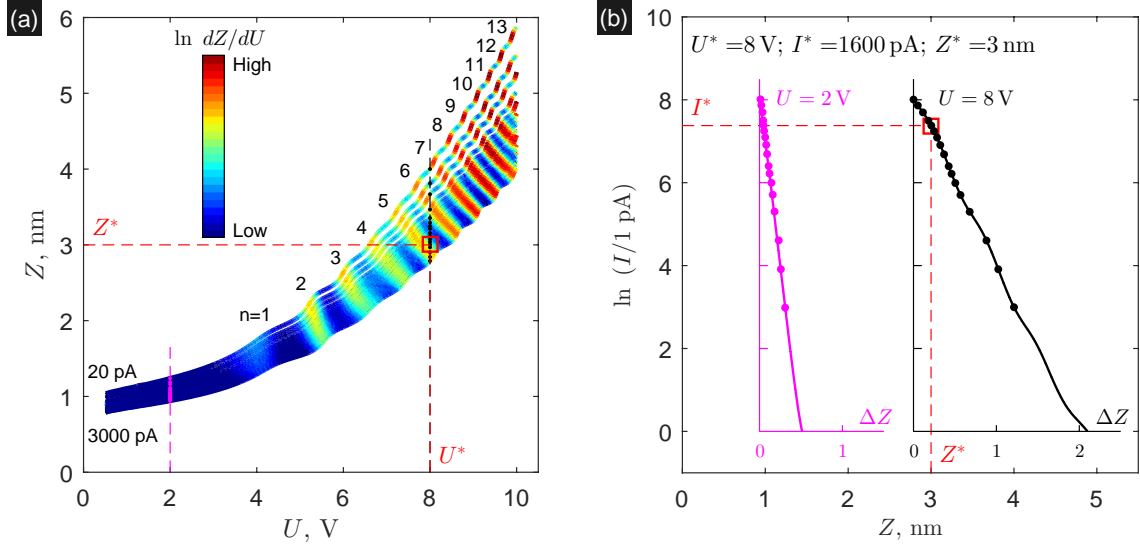

**Figure S4.** (color online) Diagrams illustrating the principle of the mutual adjustment of the  $Z-U$  dependences acquired in the regime of constant current and  $I-\Delta Z$  dependences acquired in the regime of constant voltage: **(a)** Series of the  $h-U$  dependences acquired for different tunneling currents:  $\langle I \rangle = 20, 50, 100, 200, 300, 400, 500, 600, 800, 1000, 1200, 1400, 1600, 1800, 2200, 2600$  and  $3000$  pA (from top to bottom). The color of the points is proportional to  $\ln dZ/dU$ . All these curves are slightly shifted upward and downward (about  $0.05$  nm or less to compensate vertical thermal drift and creep effect of the piezoscanner) in such a way to get the correct dependence of  $\ln I$  on  $\Delta Z$  for the given bias  $U^*$  (black dots in the panel b); this particular adjustment is performed for  $U^* = 8$  V,  $I^* = 1600$  pA,  $Z^* = 3$  nm (marked by  $\square$ ). **(b)** Purple and black solid lines are the dependences of  $\ln I$  on  $\Delta Z$ , acquired during current-distance spectroscopy measurements for  $U = +2$  and  $+8$  V, correspondingly. Purple and black dots represent the cross-sectional views for the data shown in the panel a along the dashed vertical lines for  $U = +2$  and  $+8$  V, respectively. Almost perfect agreement between different kinds of measurements in the panel b ensures the correctness of the visualization of the data in the panel a.

### The estimate of the energy of FER based on the quasi-classical WKB approximation

We would like to consider the simplest quasi-classical 1D model and calculate the energy and spatial structure of the localized states in the linearly increasing potential. This consideration is relevant for the particular cases of (i) planar structure with a tunneling barrier of constant width or (ii) very blunt STM-tip above the sample surface. This model seems to be helpful for discovering the periodic nature of the quantized heights  $Z_n$  attributed to the  $n$ -th field-emission resonances.

We start with the reproduction of the theoretical considerations, concerning the estimate for the positions of the FER and briefly presented in our recent paper (Aladyshkin, J. Phys.: Condens. Matt. **32**, 435001 (2020)), in more details since it can be of methodological interest.

The reflection coefficient from the flat surface of the sample depends on the energy. It is worth to note that the amplitude of the reflection coefficient can be equal to unity if  $E$  belongs to the forbidden energy gap of bulk crystal. Such 100% reflection ability explains the formation of the slow-decaying quasi-stationary electronic states localized above the sample in a linearly increasing potential. It allows us to consider an effective triangular

potential well (black solid line in Fig. S5a)

$$U_{pot}^{(2)}(z) = \begin{cases} \infty & \text{for } z < 0, \\ U^* + F^* \cdot z & \text{for } z \geq 0; \end{cases} \quad (\text{S3})$$

instead of trapezoidal potential barrier

$$U_{pot}^{(1)}(z) = \begin{cases} -|e|U & \text{for } z < 0; \\ U^* + F^* \cdot z & \text{for } 0 \leq z \leq Z; \\ 0 & \text{for } z > Z, \end{cases} \quad (\text{S4})$$

Here  $E_F$  is the Fermi energy of both electrodes, since the sample and the tip are in electrical contact, what equalizes the Fermi levels of the electrodes;  $U$  is the electric potential of the sample with respect to the tip,  $U^* = E_F + W_s - |e|U$  is the bias-shifted potential energy at the sample surface (at  $z \rightarrow 0^+$ ),  $W_s$  and  $W_t$  are the work function for electrons of the sample and the tip, correspondingly;  $F^* = (|e|U + \Delta W)/Z$  is the gradient of the potential energy which is proportional to the effective electric field above the surface,  $\Delta W = W_t - W_s$  accounts for the Volta contact potential due to the difference in the work functions, and  $Z$  is the distance between the STM tip and the sample surface.

We start with the substitution of the quasi-classical momentum  $p(z) = \sqrt{2m_0(E - U_{pot}^{(2)}(z))}$  into the Bohr-Sommerfeld quantization rule

$$\frac{1}{\pi\hbar} \int_a^b p(z) dz = m + \gamma, \quad m = 0, 1, \dots \quad (\text{S5})$$

where  $a = 0$  and  $b = (E - U^*)/F^*$  are classical turning points,  $m_0$  is the mass of free electron,  $m$  is the integer index, the numerical coefficient  $\gamma$  is close to  $3/4$  due to the presence of the impenetrable barrier at  $z = 0$ . We can introduce the index  $n = m + 1$  for convenience. After integration, we obtain the discrete energy spectrum

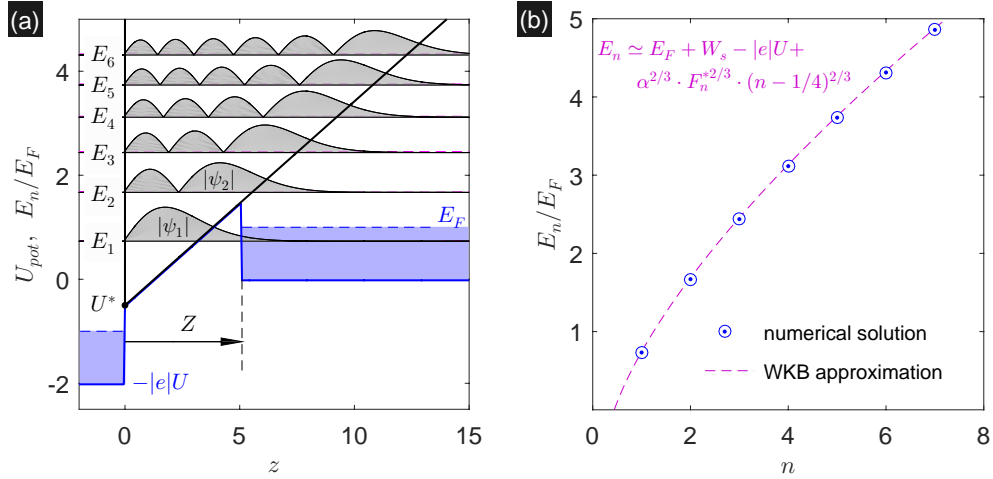

**Figure S5.** (color online) **(a)** The model profiles of the potential energy in the form of the trapezoidal barrier  $U_{pot}^{(1)}(z)$  (blue solid line) and triangular potential well  $U_{pot}^{(2)}(z)$  (black solid line). Thin black and purple horizontal lines are the eigen-energies of Eq. (S12) obtained numerically and analytically, correspondingly, for the following parameters  $W_s/E_F = 0.5$ ,  $|e|U/E_F = 2$  and  $\Delta W = 0$ . The difference between the analytical and numerical solutions for  $E_n$  are less than 2% and practically invisible in this scale. The shaded oscillatory patterns are the eigenfunctions of the Schrödinger equation (S12) calculated numerically for electron in the triangular potential well. **(b)** Comparison of the eigen-energies  $E_n$  obtained analytically [dashed line, Eq. (S9)] and numerically [ $\odot$ , Eq. (S12)] for  $W_s/E_F = 0.5$ ,  $|e|U/E_F = 2$  and  $\Delta W = 0$ .

for the electrons localized in the triangular potential well

$$E_n = U^* + \left\{ \frac{3}{2} \frac{\pi \hbar}{\sqrt{2m_0}} F_n^* \cdot \left( n - \frac{1}{4} \right) \right\}^{2/3} =$$

$$= E_F + W_s - |e|U + \left\{ \frac{3}{2} \frac{\pi \hbar}{\sqrt{2m_0}} F_n^* \cdot \left( n - \frac{1}{4} \right) \right\}^{2/3}, \quad n = 1, 2, \dots \quad (\text{S6})$$

Since the process of resonant tunnelling starts when the energy of the state localized in the area between the emitter (tip) and collector (sample) reaches the Fermi energy of the tip ( $E_n \simeq E_F$ ), we come to the relationship

$$|e|U_n \simeq W_s + \left( \frac{3}{2} \frac{\pi \hbar}{\sqrt{2m_0}} \right)^{2/3} F_n^{*2/3} \left( n - \frac{1}{4} \right)^{2/3}, \quad n = 1, 2, \dots \quad (\text{S7})$$

The quasi-classical wave function of the electron localized in the triangular potential well near the right turning point  $z = b$  can be written in the following form

$$\psi_n(z) \simeq \frac{C}{\sqrt{p(z)}} \cos \left( \frac{1}{\hbar} \int_z^b p(z) dz - \frac{\pi}{4} \right) \simeq$$

$$\simeq \frac{C}{\sqrt{2m_0(E_n - U^* - F_n^* z)}} \cos \left( \frac{2}{3F_n^*} \frac{\sqrt{2m_0}}{\hbar} (E_n - U^* - F_n^* z)^{3/2} - \frac{\pi}{4} \right). \quad (\text{S8})$$

It is easy to see that the wave function at the left turning point  $z = 0$  is equal to zero provided that the argument of the cosine function is equal to  $-\pi/2 + \pi n$

$$\frac{2}{3} \frac{\sqrt{2m_0}}{\hbar F_n^*} (E_n - U^*)^{3/2} - \frac{\pi}{4} \simeq -\frac{\pi}{2} + \pi n.$$

This equation is equivalent to the relationship (S6).

For the comparison of the analytic expression (S7) with the results of numerical simulations is it convenient to introduce the dimensionless parameters: the reduced energy  $\varepsilon = E/E_F$ , the reduced bias voltage  $u = |e|U/E_F$ , the reduced work function  $w_s = W_s/E_F$  and  $\Delta w = \Delta W_s/E_F$  as well as the reduced coordinate  $z' = z/L$  and the reduced barrier width  $h' = Z/L$ , where  $E_F$  is the natural energy scale and  $L = \sqrt{\hbar^2/(2m_0 E_F)}$

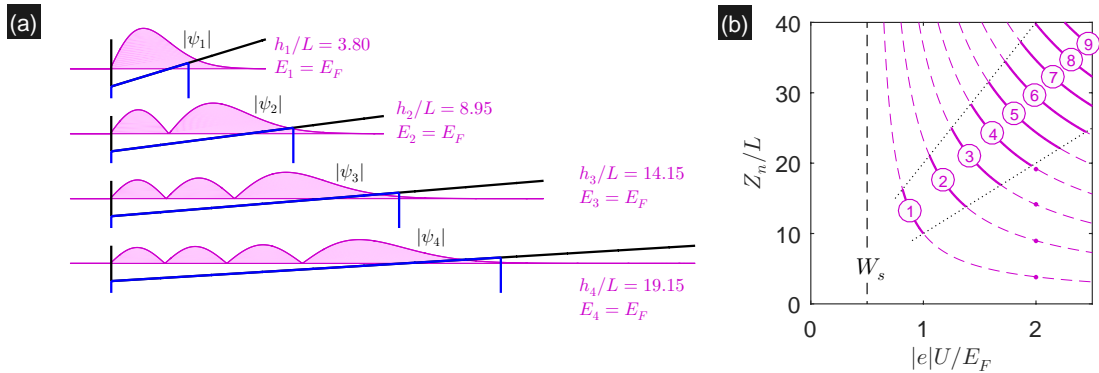

**Figure S6.** (color online) **(a)** The shaded oscillatory patterns are the eigenfunctions of the Schrödinger equation (S12) satisfying the criterion of the resonant tunneling  $E_n \simeq E_F$ . **(b)** The set of the quantized height  $h_n/L$  as a function of the dimensionless bias  $|e|U/E_F$  obtained analytically by means of Eq. (S11). Two dotted lines depict schematically the range of experimentally accessible current values (compare this plot and Fig. 4a of the main paper).

is the length scale. The expressions (S6) and (S7) can be written in the dimensionless form

$$\varepsilon_n = 1 + w_s - u + \left(\frac{3}{2}\pi\right)^{2/3} \frac{(u + \Delta w)^{2/3}}{h'^{2/3}} \left(n - \frac{1}{4}\right)^{2/3}. \quad (\text{S9})$$

and

$$u_n \simeq w_s + \left(\frac{3}{2}\pi\right)^{2/3} \frac{(u_n + \Delta w)^{2/3}}{h_n'^{2/3}} \left(n - \frac{1}{4}\right)^{2/3}. \quad (\text{S10})$$

By expressing  $h'_n$  via  $u_n$  we get the dimensionless relationship for the  $n$ -th resonant value for the barrier width as a function of the bias voltage

$$\frac{h_n}{L} \simeq \frac{3}{2}\pi \frac{(u_n + \Delta w)}{(u_n - w_s)^{3/2}} \left(n - \frac{1}{4}\right), \quad n = 1, 2, \dots \quad (\text{S11})$$

It means that in this model the proportions  $h_1 : h_2 : h_3 \dots$  for the given voltage has the universal form  $3 : 7 : 11 \dots$

The problem for the determination of the real-valued eigenfunctions  $\psi_n(z)$  and eigenvalues  $E_n$  for the particle trapped in the linearly increasing potential  $U_{pot}^{(2)}$  can be formulated in the dimensionless form as follows

$$-\frac{d^2}{dz'^2} \psi_n(z') + \left\{ (1 + w_s - u) + (u + \Delta w) \cdot \frac{z'}{h'} \right\} \psi_n(z') = \varepsilon_n \psi_n(z'), \quad (\text{S12})$$

$$\text{Boundary conditions: } \psi_n \Big|_{z'=0} = 0 \quad \text{and} \quad \psi_n \Big|_{z'=\infty} = 0.$$
